# Supplementary material for: Representation Learning for cold-start recommendation
Source: arXiv:1412.7156 source file (2015-06-22)
Supplement: Supplementary file 1 [file additional.tex]

\appendix

\newpage

\begin{figure}
\centering
\begin{subfigure}{.5\textwidth}
  \centering
  \includegraphics[width=0.9\linewidth]{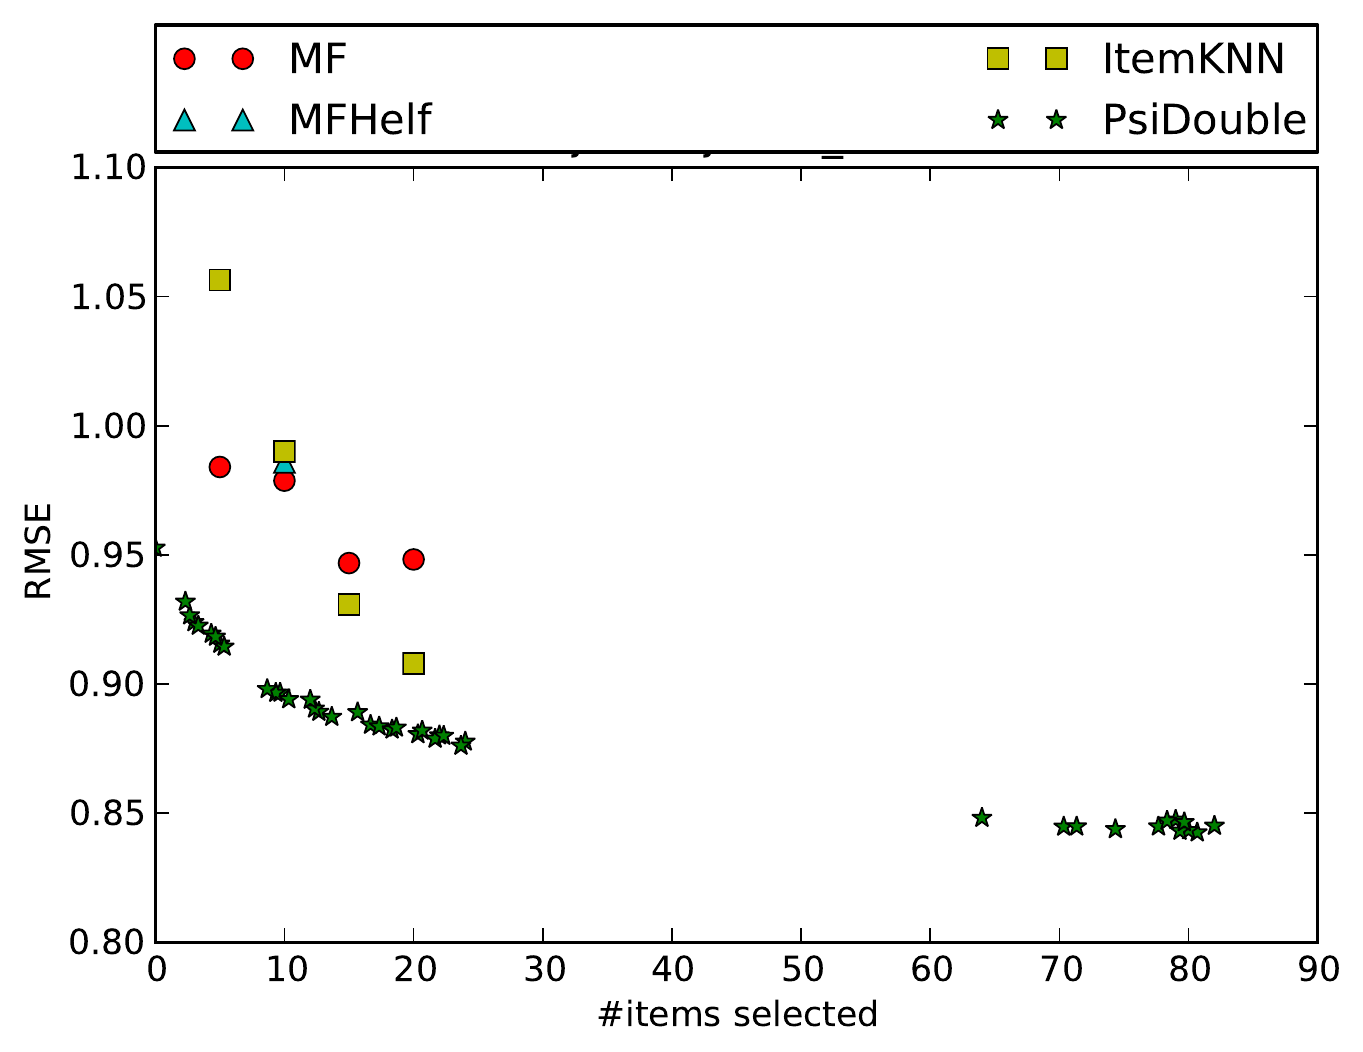}
  \caption{RMSE}
  \label{fig:jester_RMSE}
\end{subfigure}%
\begin{subfigure}{.5\textwidth}
  \centering
  \includegraphics[width=0.9\linewidth]{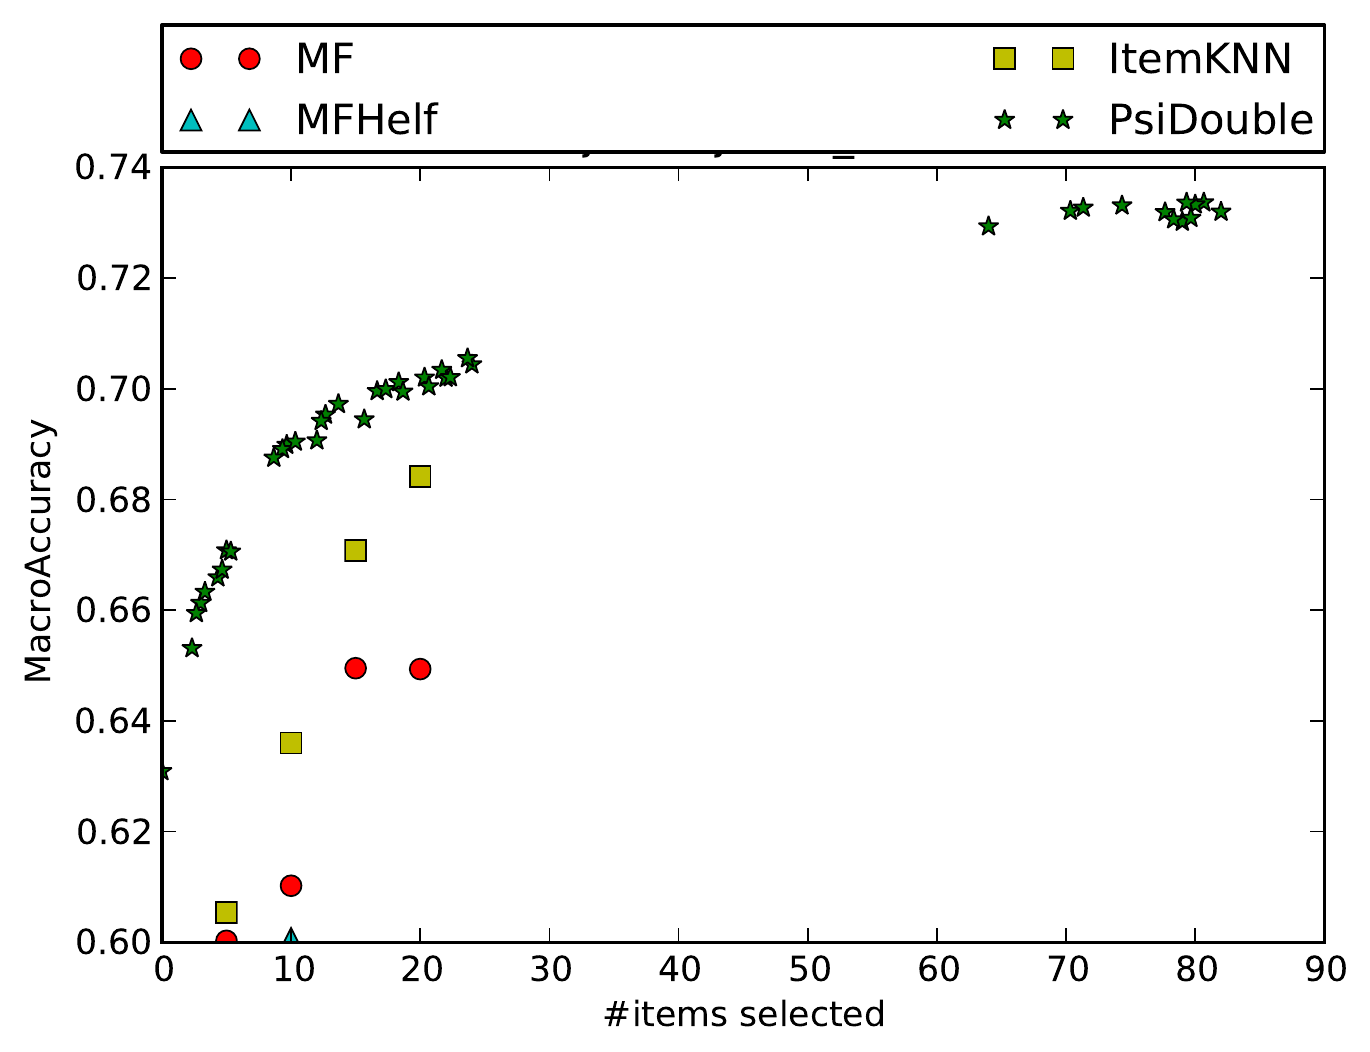}
  \caption{Accuracy}
  \label{fig:jester_Accu}
\end{subfigure}
\caption{Dataset : \textbf{Jester} }
\label{fig:jester_alphadouble}
\end{figure}

\begin{figure}
\centering
\begin{subfigure}{.5\textwidth}
  \centering
  \includegraphics[width=0.9\linewidth]{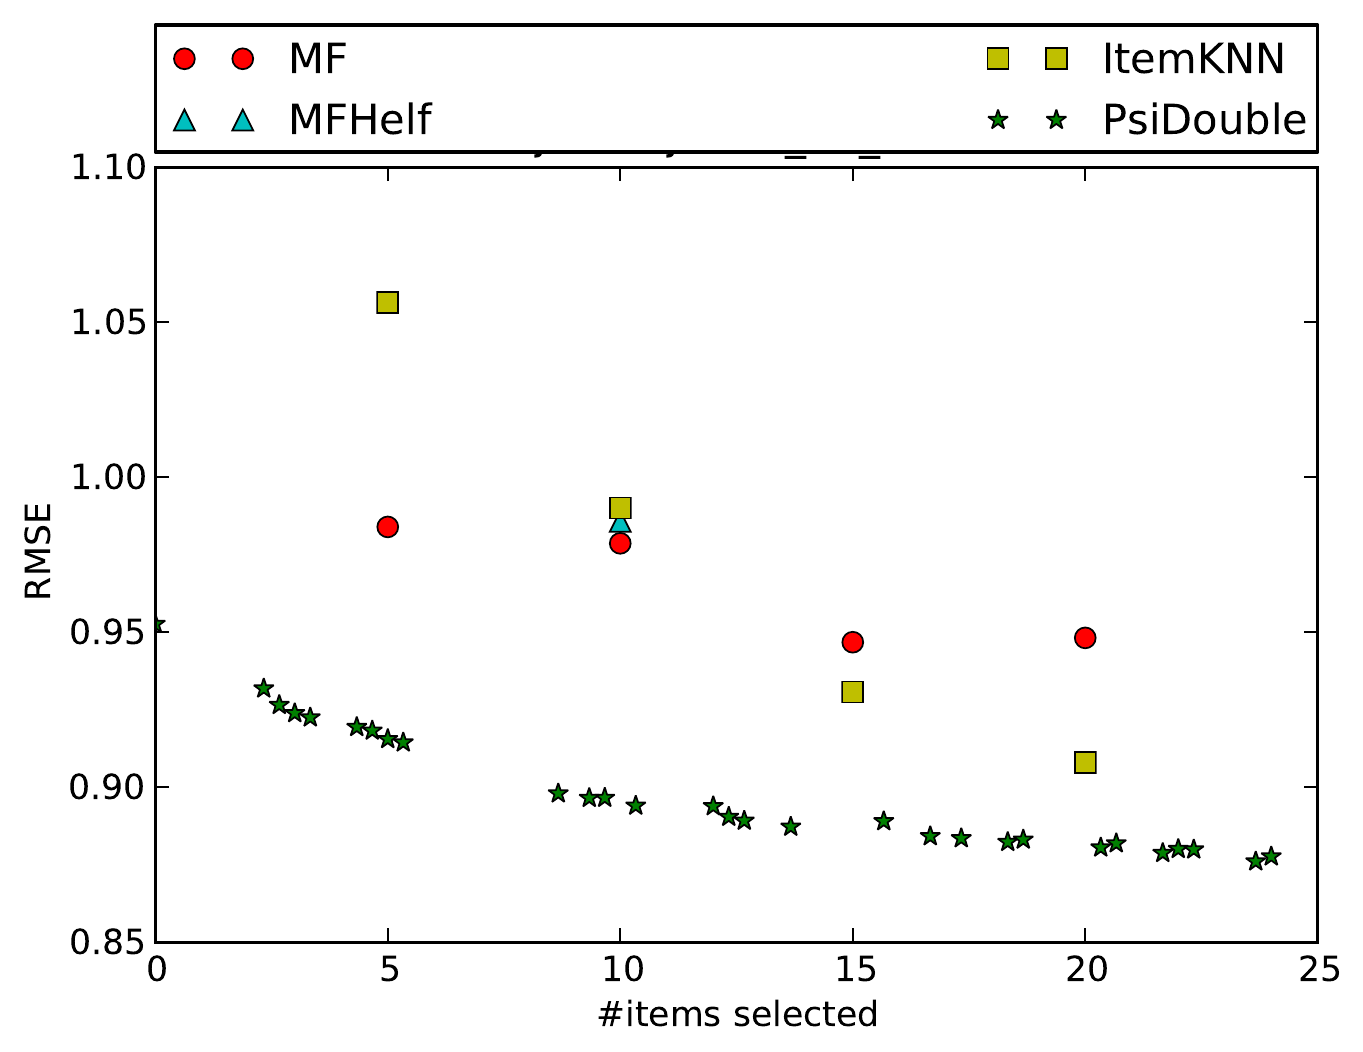}
  \caption{RMSE}
  \label{fig:jester_30_RMSE}
\end{subfigure}%
\begin{subfigure}{.5\textwidth}
  \centering
  \includegraphics[width=0.9\linewidth]{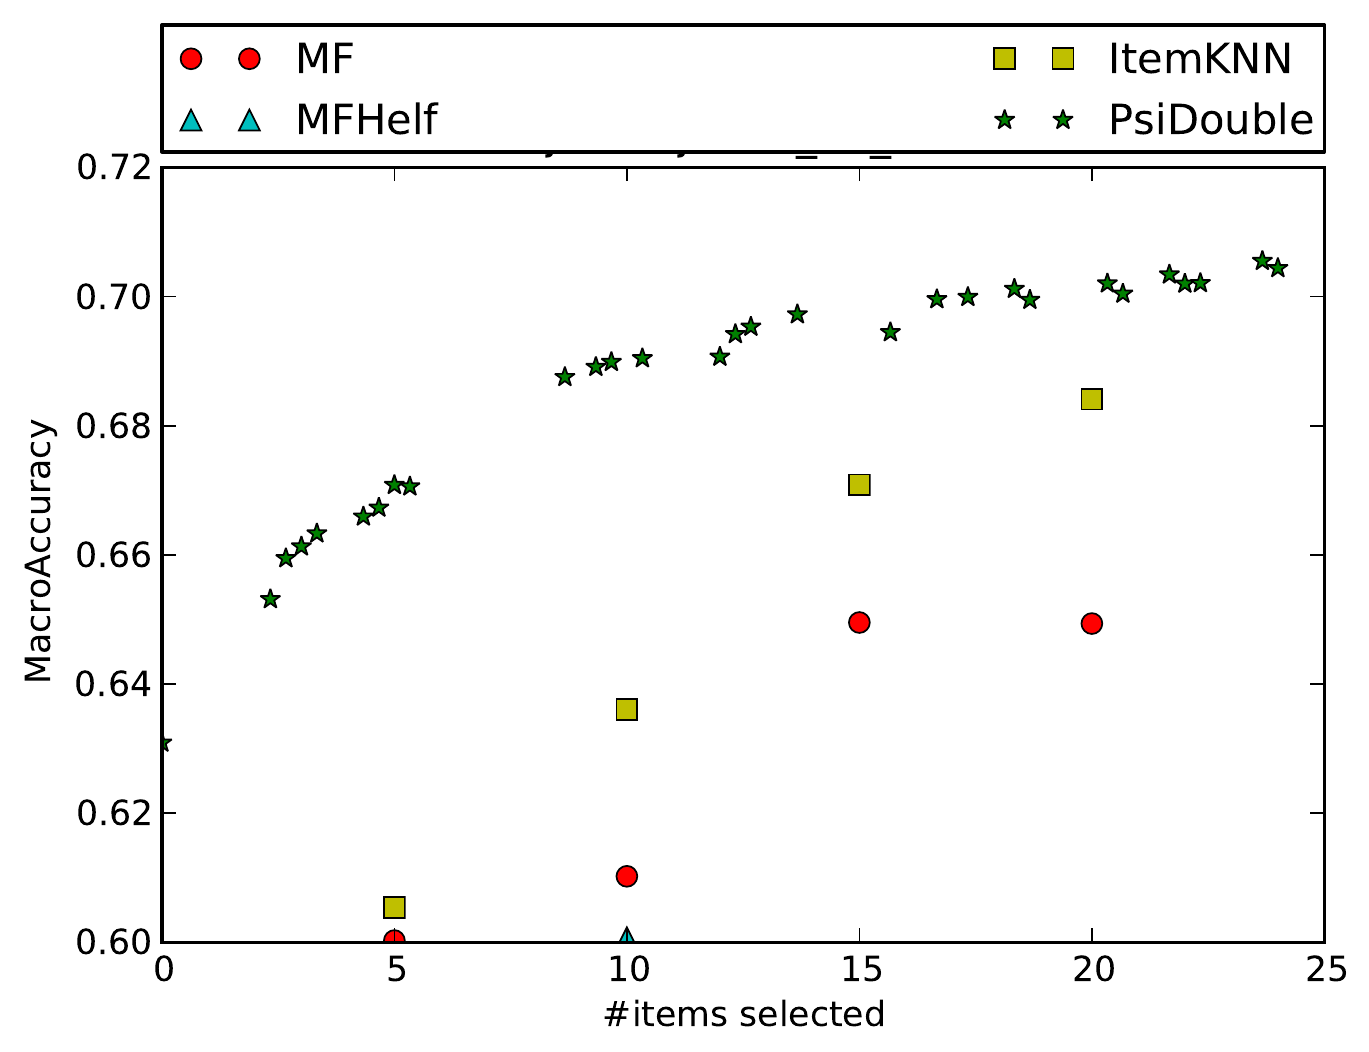}
  \caption{Accuracy}
  \label{fig:jester_30_Accu}
\end{subfigure}
\caption{Dataset : \textbf{Jester} }
\label{fig:jester_alphadouble}
\end{figure}

\begin{figure}
\centering
\begin{subfigure}{.5\textwidth}
  \centering
  \includegraphics[width=0.9\linewidth]{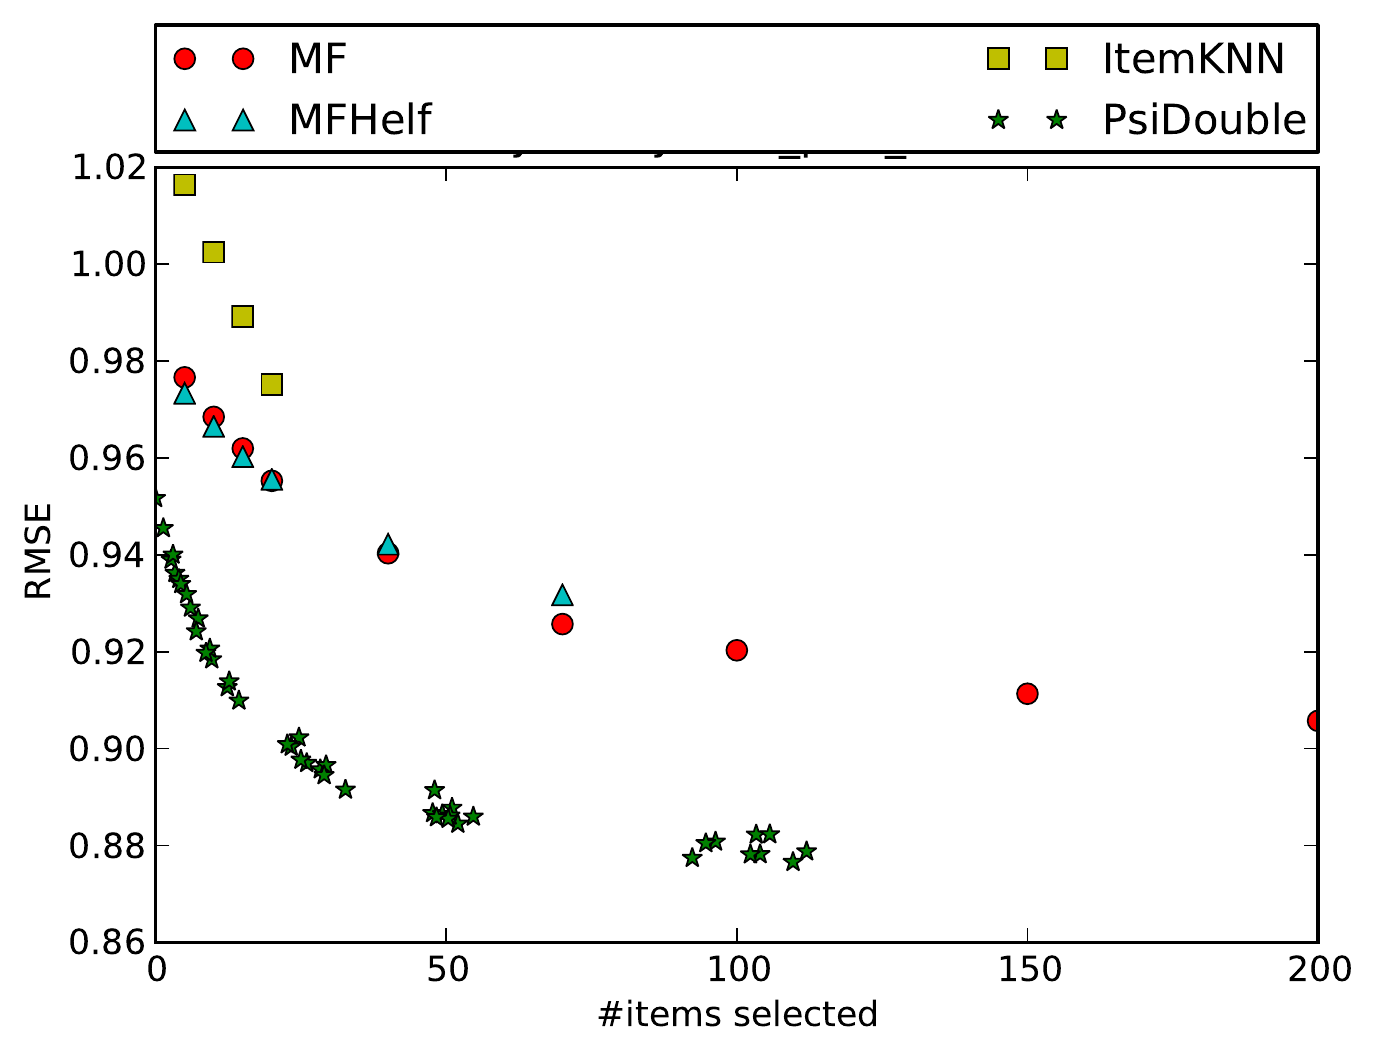}
  \caption{RMSE}
  \label{fig:yahoo_RMSE}
\end{subfigure}%
\begin{subfigure}{.5\textwidth}
  \centering
  \includegraphics[width=0.9\linewidth]{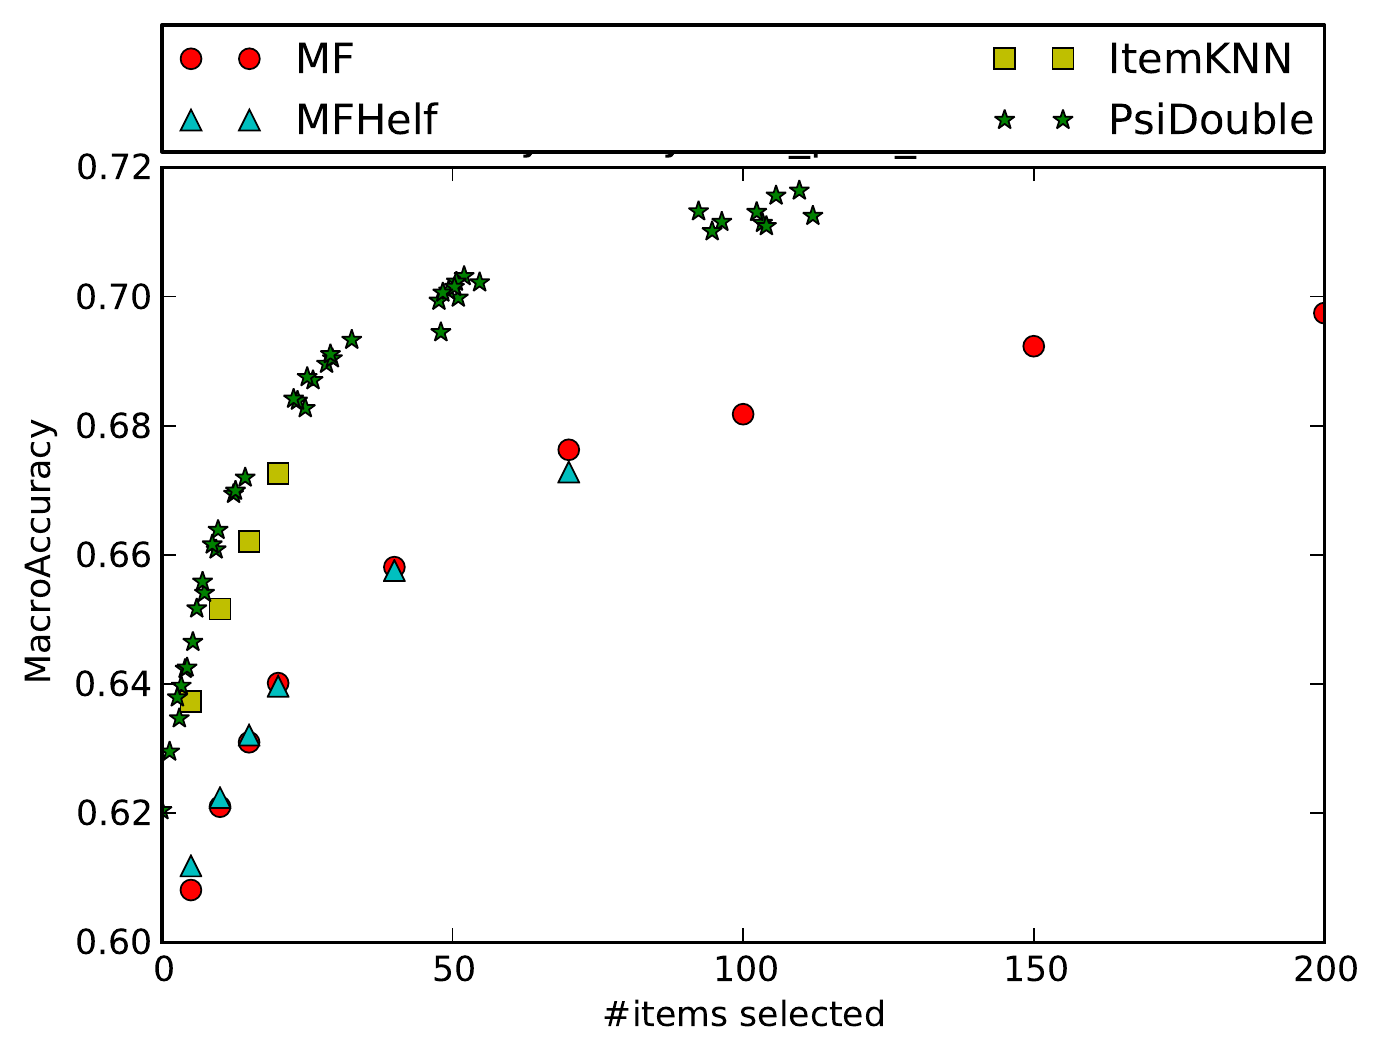}
  \caption{Accuracy}
  \label{fig:yahoo_Accu}
\end{subfigure}
\caption{Dataset : \textbf{Yahoo} }
\label{fig:ml1M_alphadouble}
\end{figure}

\begin{figure}
\centering
\begin{subfigure}{.5\textwidth}
  \centering
  \includegraphics[width=0.9\linewidth]{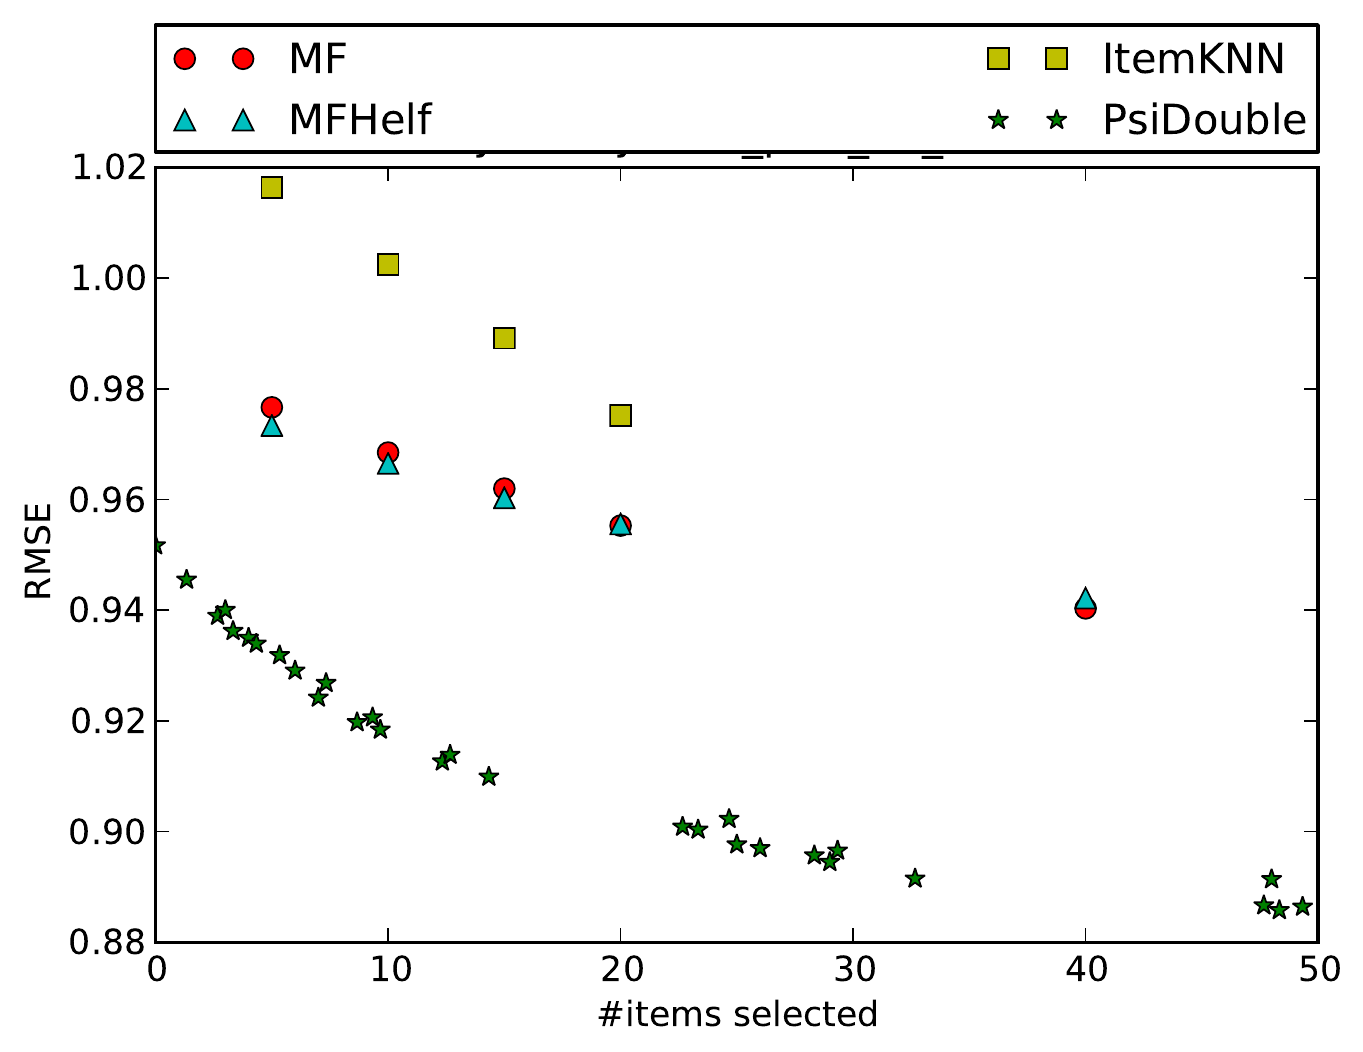}
  \caption{RMSE}
  \label{fig:yahoo_50_RMSE}
\end{subfigure}%
\begin{subfigure}{.5\textwidth}
  \centering
  \includegraphics[width=0.9\linewidth]{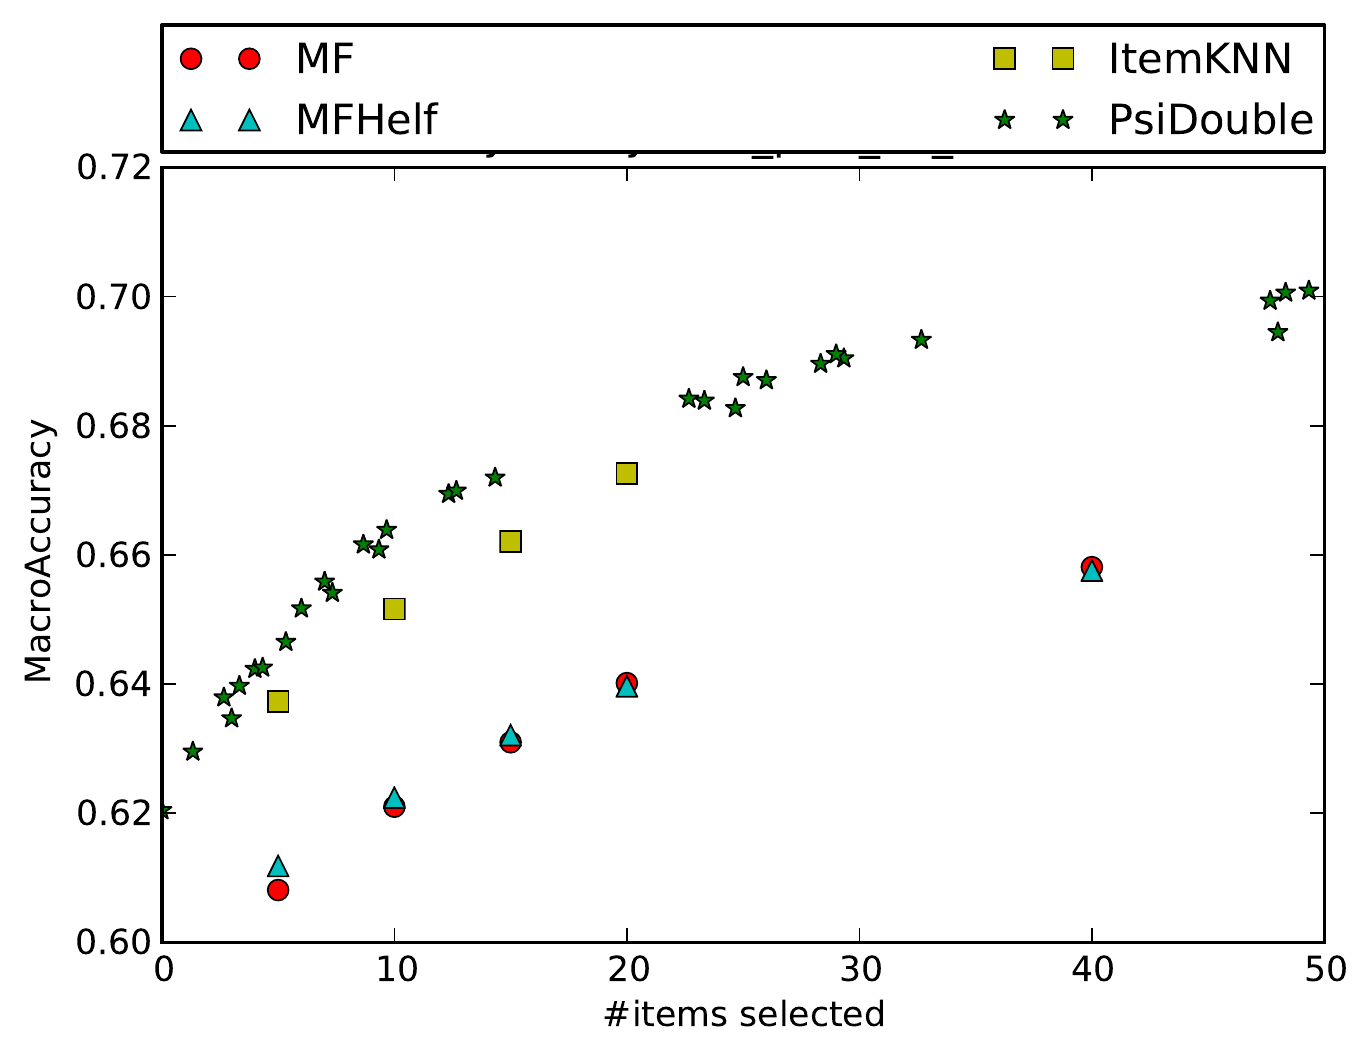}
  \caption{Accuracy}
  \label{fig:yahoo_50_Accu}
\end{subfigure}
\caption{Dataset : \textbf{Yahoo} }
\label{fig:ml1M_alphadouble}
\end{figure}

\begin{figure}
\centering
\begin{subfigure}{.5\textwidth}
  \centering
  \includegraphics[width=0.9\linewidth]{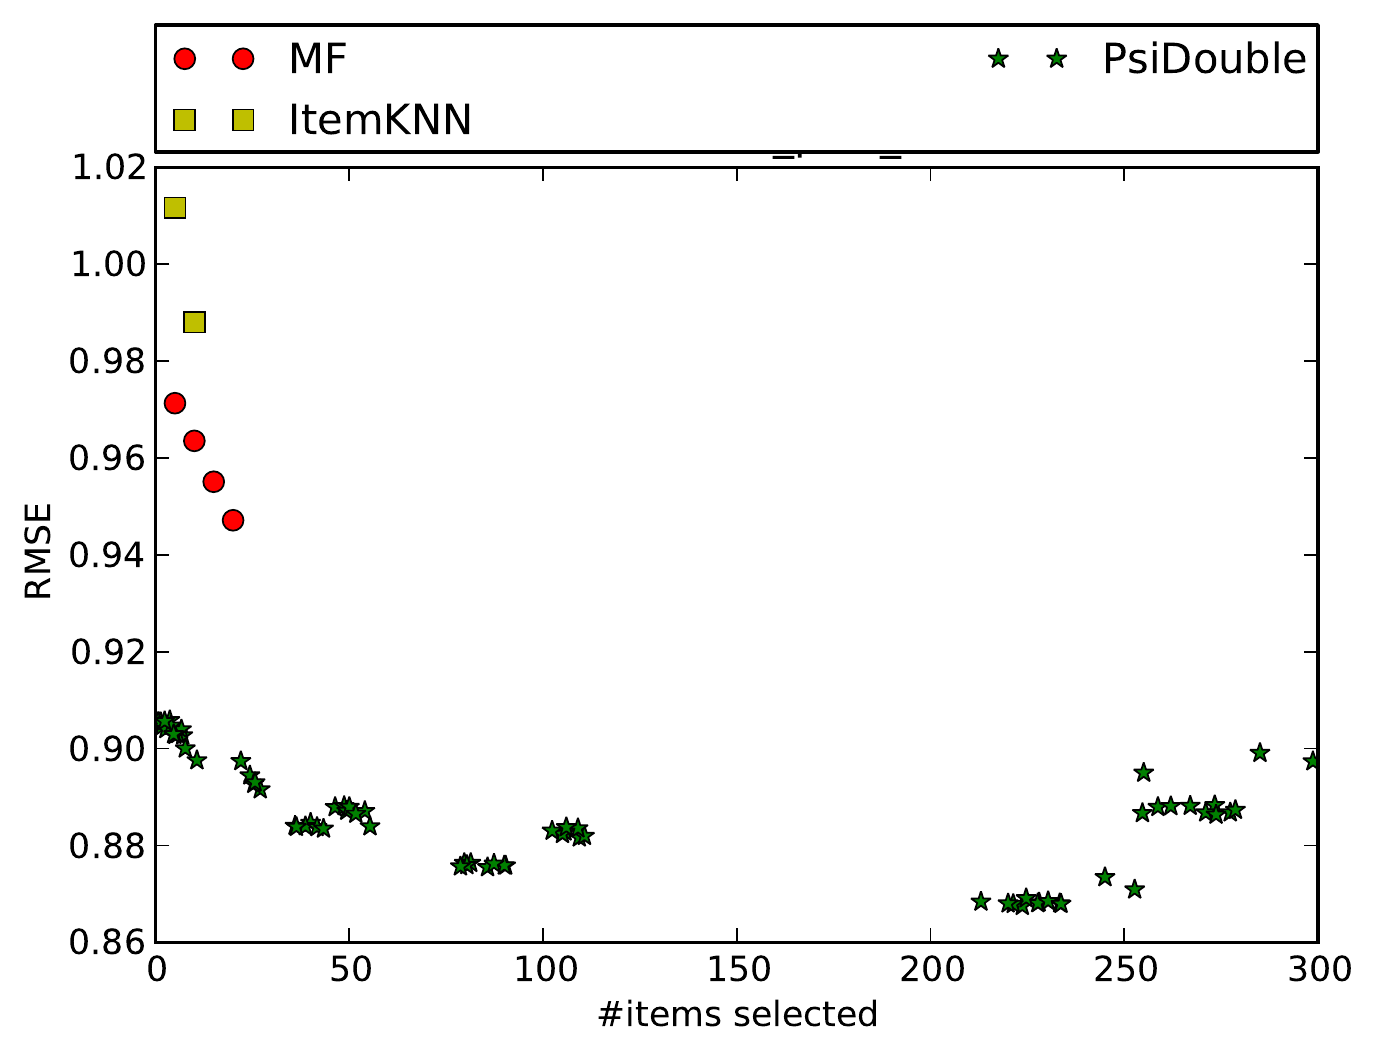}
  \caption{RMSE}
  \label{fig:ml1M_RMSE}
\end{subfigure}%
\begin{subfigure}{.5\textwidth}
  \centering
  \includegraphics[width=0.9\linewidth]{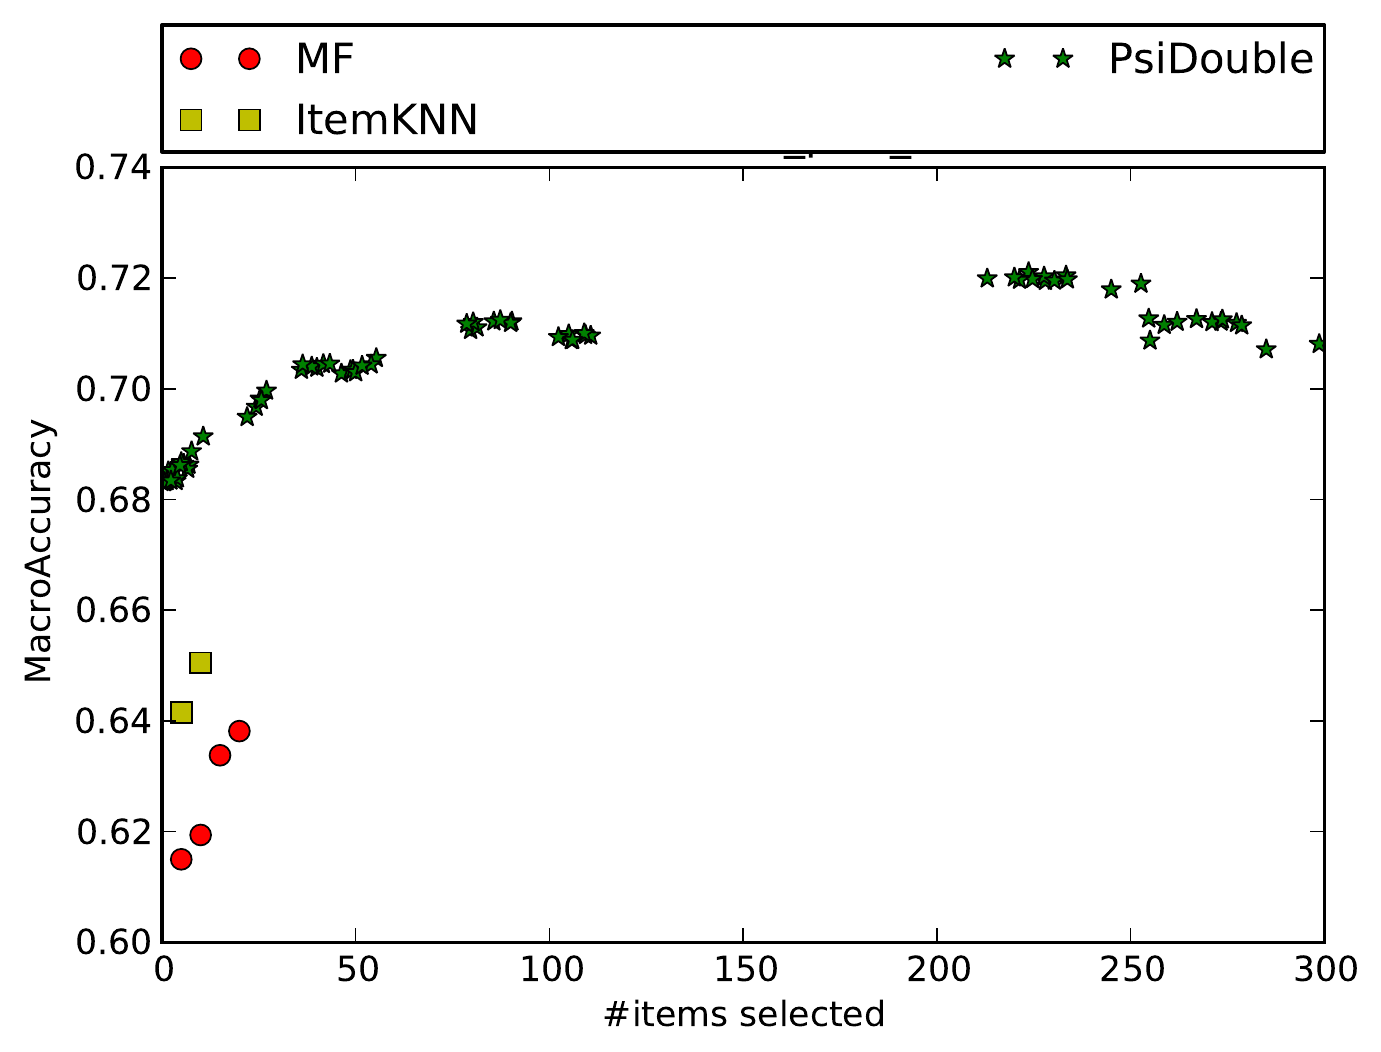}
  \caption{Accuracy}
  \label{fig:ml1M_Accu}
\end{subfigure}
\caption{Dataset : \textbf{MovieLens 1M} }
\label{fig:ml1M_alphadouble}
\end{figure}

\begin{figure}
\centering
\begin{subfigure}{.5\textwidth}
  \centering
  \includegraphics[width=0.9\linewidth]{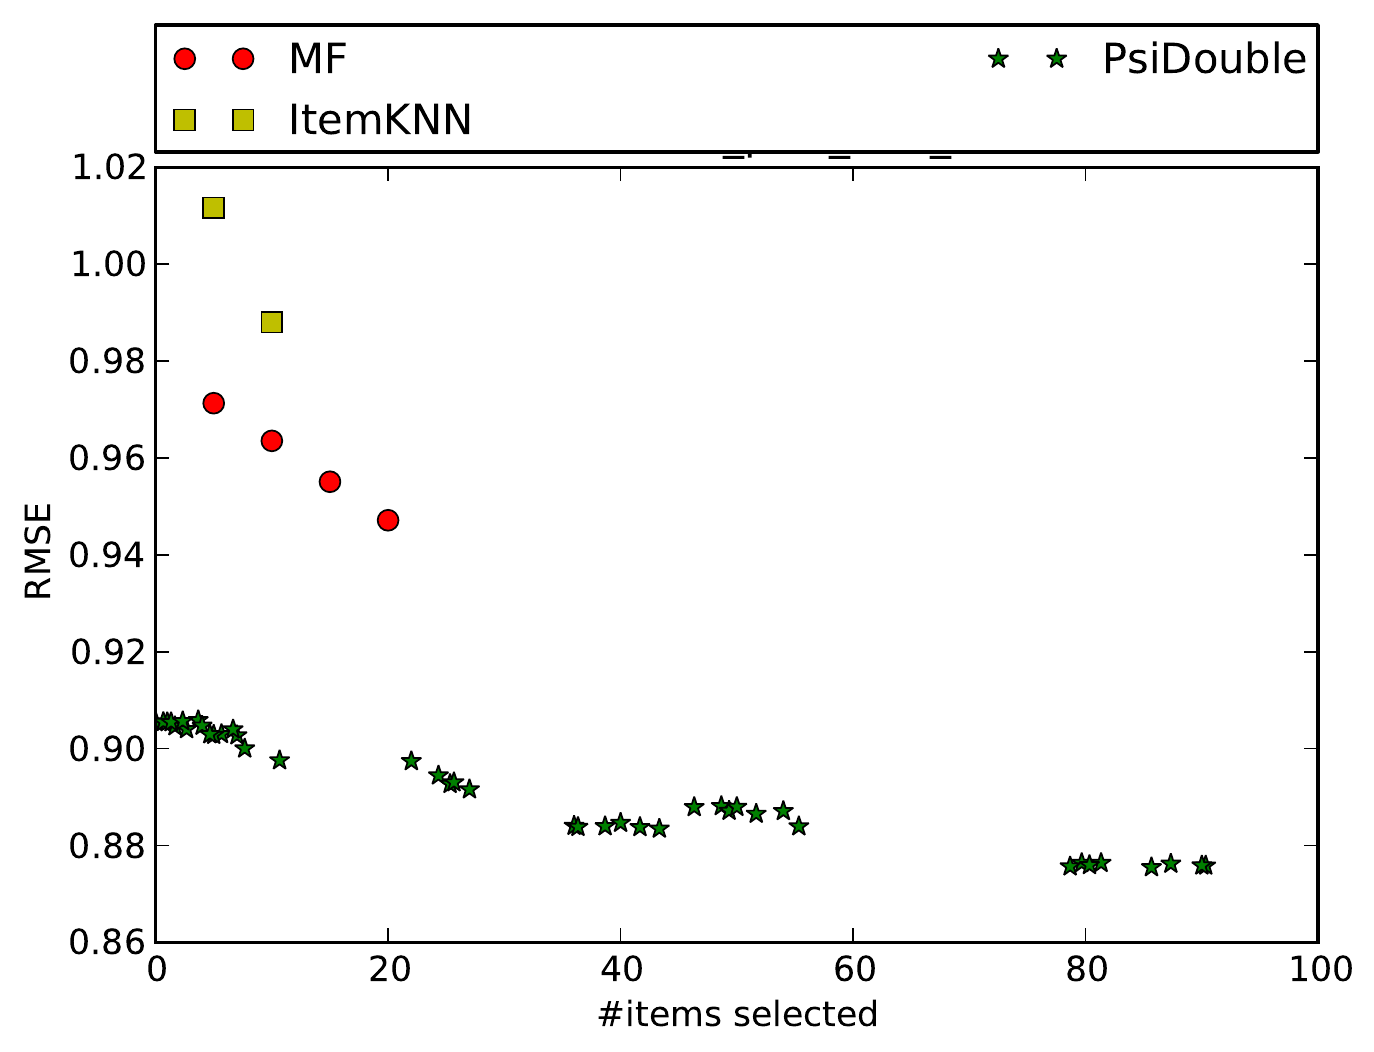}
  \caption{RMSE}
  \label{fig:ml1M_100_RMSE}
\end{subfigure}%
\begin{subfigure}{.5\textwidth}
  \centering
  \includegraphics[width=0.9\linewidth]{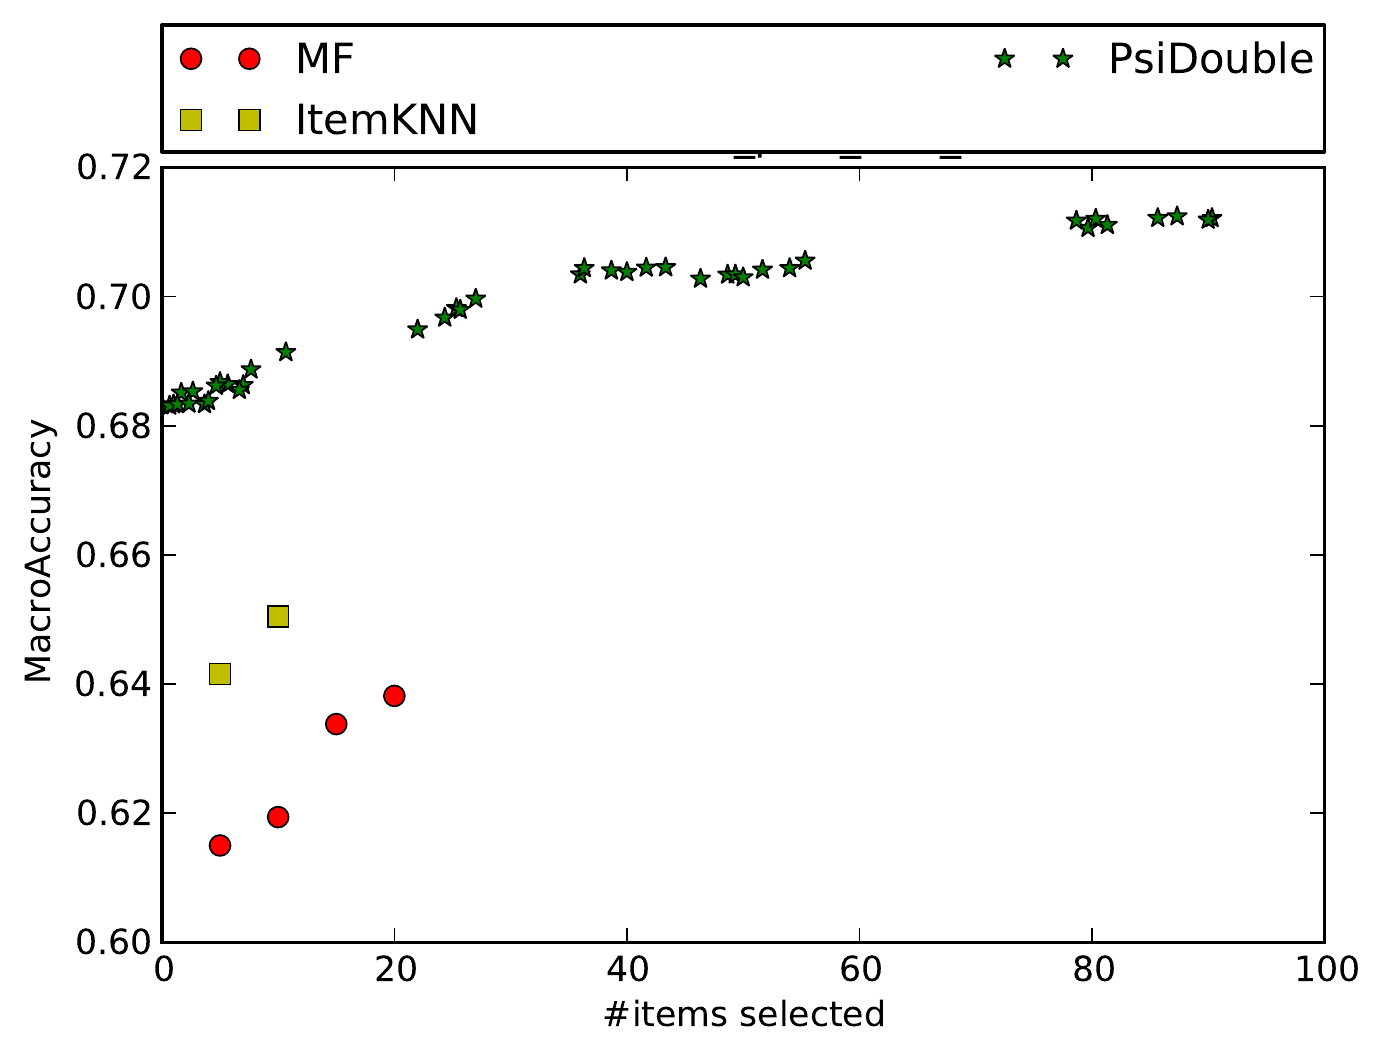}
  \caption{Accuracy}
  \label{fig:ml1M_100_Accu}
\end{subfigure}
\caption{Dataset : \textbf{MovieLens 1M} }
\label{fig:ml1M_alphadouble}
\end{figure}

\begin{table}
\begin{center}

\begin{tabular}{|l|l|c|} \hline 
Movie & Genre & $\alpha$ \\\hline
    Pleasantville (1998)& Comedy& 0.396737 \\
Mission: Impossible (1996)& Action|Adventure|Mystery& 0.384718 \\
Star Wars: Episode VI - Return of the Jedi (1983)& Action|Adventure|Romance|Sci-Fi|War& 0.252651\\
Patriot Games (1992)& Action|Thriller& 0.346994 \\
Lethal Weapon 3 (1992)& Action|Comedy|Crime|Drama& 0.413058  \\
Men in Black (1997)& Action|Adventure|Comedy|Sci-Fi& 0.412301 \\
Pulp Fiction (1994)& Crime|Drama& 0.317951 \\
Twelve Monkeys (1995)& Drama|Sci-Fi& 0.320635 \\
Crimson Tide (1995)& Drama|Thriller|War& 0.21444 \\
Mask, The (1994)& Comedy|Crime|Fantasy& 0.405714 \\
Back to the Future (1985)& Comedy|Sci-Fi& 0.351937 \\
Star Wars: Episode I - The Phantom Menace (1999)& Action|Adventure|Fantasy|Sci-Fi& 0.332822 \\
King Kong (1933)& Action|Adventure|Horror& 0.467331 \\
Who Framed Roger Rabbit? (1988)& Adventure|Animation|Film-Noir& 0.337147 \\
Rocky Horror Picture Show, The (1975)& Comedy|Horror|Musical|Sci-Fi& 0.428631 \\
Stargate (1994)& Action|Adventure|Sci-Fi& 0.308211 \\
Fantasia (1940)& Animation|Children's|Musical& 0.230316 \\
Time Bandits (1981)& Adventure|Fantasy|Sci-Fi& 0.341268 \\
Stand by Me (1986)& Adventure|Comedy|Drama& 0.393858 \\
Lost World: Jurassic Park, The (1997)& Action|Adventure|Sci-Fi|Thriller& 0.316492 \\
League of Their Own, A (1992)& Comedy|Drama& 0.347843 \\
Predator (1987)& Action|Sci-Fi|Thriller& 0.364581 \\
Jewel of the Nile, The (1985)& Action|Adventure|Comedy|Romance& 0.349509 \\
Say Anything... (1989)& Comedy|Drama|Romance& 0.425995 \\
West Side Story (1961)& Musical|Romance& 0.524218 \\
Broadcast News (1987)& Comedy|Drama|Romance& 0.472813 \\
Outbreak (1995)& Action|Drama|Thriller& 0.269675 \\ \hline
\end{tabular}
\end{center}
\caption{MovieLens 1M - An example of selected items for the interview process}
\label{tab:interview}
\end{table}
